# Supplementary material for: MultiLegalSBD: A Multilingual Legal Sentence Boundary Detection Dataset
Source: arXiv:2305.01211 source file (2023-05-02)
Supplement: Supplementary file 1 [file Appendix.tex]

\iffalse %delete this and \fi at the end to uncomment appendix

\clearpage
\section{Appendix}



\subsection{Dataset Sources}
\label{ss:datasetSources}

\begin{description}
    \item \href{https://wipolex.wipo.int/en/main/home}{Wipolex}
    \item \href{http://www.jus.unitn.it/cardozo/Obiter_Dictum/}{Jus.unitn.it}
    \item \href{https://huggingface.co/datasets/swiss_judgment_prediction}{\ac{SJP}}
    \item \href{https://huggingface.co/datasets/joelito/Multi_Legal_Pile}{\ac{MLP}}
    \item \href{https://github.com/sebischair/Legal-Sentence-Boundary-Detection}{\citet{Glaser}}
    \item \href{https://github.com/jsavelka/sbd_adjudicatory_dec}{\citet{Savelka}}
\end{description}

\subsection{CRF Feature Representation}
\label{app:CRFFeature}
A sample representation of "en" in the sequence "C'est en outre ...":
\{\\
'bias': 1.0, '0:lowercase': 'en', '0:lower': True, '0:upper': False,\\
'0:numeric': False, '0:special': 'No', '0:sign': 'cc', '0:length': 2,\\
'0:BOS': False, '0:EOS': False, '-1:BOS': False, '-1:special': 'S',\\
'-1:lowercase': ' ', '-1:length': 1, '-1:sign': 'S', '-1:lower': False,\\
'-1:upper': False, '-1:number': False, '-1:space': True, '-2:BOS': False,\\
'-2:special': 'No', '-2:lowercase': 'est', '-2:length': 3,\\
'-2:sign': 'ccc', '-2:lower': True, '-2:upper': False, '-2:number': False,\\
'-2:space': False, '-3:BOS': False, '-3:special': 'Abbr',\\
'-3:lowercase': "'", '-3:length': 1, '-3:sign': 'S', '-3:lower': False,\\
'-3:upper': False, '-3:number': False, '-3:space': False, '-4:BOS': True,\\
'-4:special': 'No', '-4:lowercase': 'c', '-4:length': 1, '-4:sign': 'C',\\
'+1:EOS': False, '+1:special': 'S', '+1:lowercase': ' ', '+1:length': 1,\\
'+1:sign': 'S', '+1:lower': False, '+1:upper': False, '+1:number': False,
'+1:space': True, '+2:EOS': True, '+2:special': 'No', \\
'+2:lowercase': 'outre', '+2:length': 5, '+2:sign': 'ccccc',\\
'+2:lower': True, '+2:upper': False, '+2:number': False, '+2:space': False\\
\}


%\subsection{CRF Feature Representation Example}
%\label{lst:features}
%Sample representation of "en" in the sequence "C'est en outre ...":\\
%\\
%'bias': 1.0, '0:lowercase': 'en', '0:lower': True, '0:upper': False, '0:numeric': False, '0:special': 'No', '0:sign': 'cc', '0:length': 2, '0:BOS': False, '0:EOS': False, '-1:BOS': False, '-1:special': 'S', '-1:lowercase': ' ', '-1:length': 1, '-1:sign': 'S', '-1:lower': False, '-1:upper': False, '-1:number': False, '-1:space': True, '-2:BOS': False, '-2:special': 'No', '-2:lowercase': 'est', '-2:length': 3, '-2:sign': 'ccc', '-2:lower': True, '-2:upper': False, '-2:number': False, '-2:space': False, '-3:BOS': False, '-3:special': 'Abbr', '-3:lowercase': "'", '-3:length': 1, '-3:sign': 'S', '-3:lower': False, '-3:upper': False, '-3:number': False, '-3:space': False, '-4:BOS': True, '-4:special': 'No', '-4:lowercase': 'c', '-4:length': 1, '-4:sign': 'C', '+1:EOS': False, '+1:special': 'S', '+1:lowercase': ' ', '+1:length': 1, '+1:sign': 'S', '+1:lower': False, '+1:upper': False, '+1:number': False, '+1:space': True, '+2:EOS': True, '+2:special': 'No', '+2:lowercase': 'outre', '+2:length': 5, '+2:sign': 'ccccc', '+2:lower': True, '+2:upper': False, '+2:number': False, '+2:space': False

\subsection{Performance of baseline models}
\label{ss:baselineModelsApp}
In Tables \ref{tab:frBaseline}, \ref{tab:ESbaseline}, \ref{tab:ITbaseline}, \ref{tab:enBaseline}, \ref{tab:deBaseline} and \ref{tab:brBaseline} we report the performance of all baseline models for French, Spanish, Italian, English, German and Portuguese respectively.

\begin{table*}
\centering
\caption{Performance of baseline models on the French dataset}
\label{tab:frBaseline}
\resizebox{\columnwidth}{!}{
\begin{tabular}{l|ccc|ccc} 
\toprule
\multicolumn{1}{r|}{Type} & \multicolumn{3}{c|}{Judgements} & \multicolumn{3}{c}{Laws} \\
Model & F1 & Precision & Recall & F1 & Precision & Recall \\ 
\midrule
CoreNLP & 74.7 & 68.8 & 81.7 & 76.7 & 98.5 & 62.9 \\
NLTK & 72.5 & 65.6 & 80.9 & 75.8 & 94.8 & 63.1 \\
NLTK-train & 82.9 & 87.2 & 79.0 & 75.8 & 95.1 & 63.1 \\
Spacy & 86.6 & 83.6 & 89.9 & 67.2 & 61.3 & 74.9 \\
Stanza & 81.9 & 81.3 & 82.5 & 81.0 & 80.7 & 81.4 \\
\bottomrule
\end{tabular}}
\end{table*}


\begin{table*}
\caption{Performance of baseline models on the Spanish dataset}
\label{tab:ESbaseline}
\resizebox{\columnwidth}{!}{
\begin{tabular}{l|ccc|ccc} 
\toprule
\multicolumn{1}{r|}{Type} & \multicolumn{3}{c|}{Judgements} & \multicolumn{3}{c}{Laws} \\
Model & F1 & Precision & Recall & F1 & Precision & Recall \\ 
\midrule
CoreNLP    &       71.4 &      82.5 &   63.5 &  89.0 &      98.6 &   81.2 \\
NLTK       &       70.2 &      82.3 &   61.5 &  89.2 &      99.4 &   81.0 \\
NLTK-train &       72.1 &      89.7 &   60.4 &  81.6 &      99.9 &   69.1 \\
Spacy      &       60.0 &      79.6 &   48.4 &  70.3 &      79.9 &   62.9 \\
Stanza     &       83.2 &      81.2 &   85.5 &  90.2 &      97.7 &   84.0 \\
\bottomrule
\end{tabular}}
\end{table*}

\begin{table*}
\caption{Performance of baseline models on the Italian dataset}
\label{tab:ITbaseline}
\resizebox{\columnwidth}{!}{
\begin{tabular}{l|ccc|ccc} 
\toprule
\multicolumn{1}{r|}{Type} & \multicolumn{3}{c|}{Judgements} & \multicolumn{3}{c}{Laws} \\
Model & F1 & Precision & Recall & F1 & Precision & Recall \\ 
\midrule
CoreNLP    &       79.8 &      81.8 &   78.0 &  75.6 &      91.6 &   64.6 \\
NLTK       &       72.3 &      63.0 &   85.7 &  66.3 &      67.2 &   66.0 \\
NLTK-train &       84.8 &      86.4 &   83.2 &  77.5 &      94.1 &   66.0 \\
Spacy      &       73.9 &      63.7 &   88.5 &  73.7 &      79.5 &   69.0 \\
Stanza     &       85.7 &      86.0 &   85.6 &  87.4 &      92.2 &   83.4 \\
\bottomrule
\end{tabular}}
\end{table*}

\begin{table*}
\centering
\caption{Performance of baseline models on the English dataset}
\label{tab:enBaseline}
\begin{tabular}{l|ccc} 
\toprule
\multicolumn{1}{r|}{Type} & \multicolumn{3}{c}{Judgements} \\
Model & F1 & Precision & Recall \\ 
\midrule
CoreNLP    &       81.7 &      81.5 &   82.0 \\
NLTK       &       77.2 &      72.2 &   83.1 \\
NLTK-train &       84.9 &      87.4 &   82.6 \\
Spacy      &       79.7 &      89.0 &   72.3 \\
Stanza     &       92.3 &      95.0 &   89.8 \\
\bottomrule
\end{tabular}
\end{table*}

\begin{table*}
\centering
\caption{Performance of baseline models on the German dataset}
\label{tab:deBaseline}
\resizebox{\columnwidth}{!}{
\begin{tabular}{l|ccc|ccc} 
\toprule
\multicolumn{1}{r|}{Type} & \multicolumn{3}{c|}{Judgements} & \multicolumn{3}{c}{Laws} \\
Model & F1 & Precision & Recall & F1 & Precision & Recall \\ 
\midrule
CoreNLP    &       69.0 &      63.4 &   75.6 &  64.0 &      66.8 &   61.4 \\
NLTK       &       72.3 &      69.2 &   75.7 &  73.8 &      92.4 &   61.4 \\
NLTK-train &       74.2 &      73.0 &   75.3 &  73.5 &      91.5 &   61.4 \\
Spacy      &       87.5 &      81.8 &   94.1 &  67.0 &      59.8 &   76.1 \\
Stanza     &       72.6 &      69.1 &   76.5 &  64.7 &      65.4 &   64.0 \\
\bottomrule
\end{tabular}}
\end{table*}

\begin{table*}
\centering
\caption{Performance of baseline models on the Portuguese dataset}
\label{tab:brBaseline}
\resizebox{\columnwidth}{!}{
\begin{tabular}{l|ccc|ccc} 
\toprule
\multicolumn{1}{r|}{Type} & \multicolumn{3}{c|}{Judgements} & \multicolumn{3}{c}{Laws} \\
Model & F1 & Precision & Recall & F1 & Precision & Recall \\ 
\midrule
CoreNLP & - & - & - & - & - & - \\
NLTK       &       64.9 &      74.3 &   58.2 &  57.0 &      69.3 &   50.6 \\
NLTK-train &       71.7 &      93.4 &   58.4 &  64.3 &      97.1 &   49.9 \\
Spacy      &       59.0 &      52.5 &   67.4 &  77.7 &      90.1 &   68.9 \\
Stanza     &       88.6 &      87.6 &   89.9 &  73.4 &      90.4 &   62.2 \\
\bottomrule
\end{tabular}}
\end{table*}

\subsection{Performance of our monolingual models}
\label{ss:trainedModelsApp}
In Tables \ref{tab:FrTrained}, \ref{tab:esTrained}, \ref{tab:itTrained}, \ref{tab:enTrained} and \ref{tab:deTrained} we report the performance of our monolingual models for French, Spanish, Italian, English and German respectively.

\begin{table*}
\centering
\caption{Mean (\textpm std) performance of our models on the French dataset}
\label{tab:FrTrained}
\begin{tabular}{c|c|c|c|c|c|c|c} 
\toprule
\multicolumn{1}{c}{} &  & \multicolumn{3}{c|}{Judgements} & \multicolumn{3}{c}{Laws} \\
Model & Trained on & F1 & Precision & Recall & F1 & Precision & Recall \\ 
\midrule
\multirow{3}{*}{CRF} & Judg. & 97.94 & 97.38 & 98.50 & 73.18 & 88.09 & 62.62 \\
 & Laws & 78.45 & 84.25 & 73.40 & 98.84 & 99.54 & 98.15 \\
 & Laws + Jugd. & 98.83 & 98.24 & 99.42 & 99.18 & 99.75 & 98.64 \\ 
\hline
\multirow{3}{*}{BiLSTM-CRF} & Judg. & 97.27\textpm0.27 & 96.80\textpm0.51 & 97.74\textpm0.57 & 56.65\textpm2.99 & 63.66\textpm2.06 & 51.78\textpm6.36 \\
 & Laws & 66.07\textpm4.22 & 70.71\textpm13.56 & 63.70\textpm5.43 & 97.94\textpm0.20 & 98.47\textpm0.25 & 97.40\textpm0.27 \\
 & Laws + Jugd. & 97.03\textpm0.43 & 96.45\textpm0.67 & 97.62\textpm0.46 & 98.07\textpm0.13 & 98.84\textpm0.30 & 97.32\textpm0.14 \\ 
\hline
\multirow{3}{*}{Transformer} & Judg. & 98.24\textpm0.13 & 97.39\textpm0.26 & 99.10\textpm0.06 & 84.73\textpm1.21 & 93.44\textpm0.48 & 77.67\textpm2.15 \\
 & Laws & 92.45\textpm0.47 & 96.43\textpm0.68 & 88.79\textpm0.96 & 97.58\textpm0.40 & 98.00\textpm0.77 & 97.18\textpm0.11 \\
 & Laws + Jugd. & 98.36\textpm0.08 & 97.78\textpm0.10 & 98.95\textpm0.13 & 98.23\textpm0.22 & 99.17\textpm0.40 & 97.31\textpm0.12 \\
\bottomrule
\end{tabular}
\end{table*}

\begin{table*}
\centering
\caption{Mean (\textpm std) performance of our models on the Italian dataset}
\label{tab:itTrained}
\begin{tabular}{c|c|c|c|c|c|c|c} 
\toprule
\multicolumn{1}{c}{} &  & \multicolumn{3}{c|}{Judgements} & \multicolumn{3}{c}{Laws} \\
Model & Trained on & F1 & Precision & Recall & F1 & Precision & Recall \\ 
\midrule
\multirow{3}{*}{CRF} & Judg. & 98.50 & 98.60 & 98.41 & 95.64 & 96.42 & 94.97 \\
 & Laws & 88.59 & 87.92 & 89.48 & 99.61 & 99.52 & 99.70 \\
 & Laws + Judg. & 98.28 & 98.41 & 98.14 & 99.52 & 99.50 & 99.54 \\ 
\hline
\multirow{3}{*}{BiLSTM-CRF} & Judg. & 95.92\textpm0.27 & 96.44\textpm 0.56 & 95.41\textpm 0.63 & 71.32\textpm 2.21 & 85.90\textpm 8.23 & 61.60\textpm 3.68 \\
 & Laws & 74.08\textpm1.21 & 87.32\textpm 3.03 & 65.12\textpm 3.14 & 98.36\textpm 0.25 & 99.20\textpm 0.20 & 97.53\textpm 0.47 \\
 & Laws + Judg. & 96.21\textpm0.19 & 97.36\textpm 0.67 & 95.11\textpm 0.66 & 98.17\textpm 0.13 & 99.08\textpm 0.15 & 97.28\textpm 0.31 \\ 
\hline
\multirow{3}{*}{Transformer} & Judg. & 97.84\textpm 0.18 & 98.17\textpm 0.28 & 97.52\textpm 0.20 & 81.82\textpm 0.85 & 76.88\textpm 1.07 & 87.65\textpm 2.13 \\
 & Laws & 89.41\textpm 0.69 & 95.35\textpm 0.48 & 84.20\textpm 1.53 & 98.81\textpm 0.49 & 99.33\textpm 0.51 & 98.29\textpm 0.48 \\
 & Laws + Judg. & 97.08\textpm 0.25 & 97.29\textpm 0.33 & 96.88\textpm 0.21 & 99.11\textpm 0.09 & 99.61\textpm 0.09 & 98.62\textpm 0.09 \\
\bottomrule
\end{tabular}
\end{table*}

\begin{table*}
\centering
\caption{Mean (\textpm std) performance of our models on the Spanish dataset}
\label{tab:esTrained}
\begin{tabular}{c|c|c|c|c|c|c|c} 
\toprule
\multicolumn{1}{c}{} &  & \multicolumn{3}{c|}{Judgements} & \multicolumn{3}{c}{Laws} \\
Model & Trained on & F1 & Precision & Recall & F1 & Precision & Recall \\ 
\midrule
\multirow{3}{*}{CRF} & Judg. & 96.98 & 98.61 & 95.40 & 98.32 & 98.91 & 97.76 \\
 & Laws & 54.34 & 65.84 & 46.44 & 99.64 & 99.52 & 99.76 \\
 & Laws + Judg. & 97.02 & 98.34 & 95.76 & 99.48 & 99.36 & 99.60 \\ 
\hline
\multirow{3}{*}{BiLSTM-CRF} & Judg. & 94.65\textpm 0.54 & 97.61\textpm 0.53 & 91.92 1.02 & 92.06\textpm 0.92 & 97.01\textpm 1.74 & 87.61\textpm 0.91 \\
 & Laws & 43.43\textpm 6.81 & 54.63\textpm 4.73 & 37.73 10.14 & 98.69\textpm 0.19 & 99.27\textpm 0.16 & 98.11\textpm 0.36 \\
 & Laws + Judg. & 95.62\textpm 0.49 & 97.53\textpm 0.65 & 93.79 0.46 & 98.94\textpm 0.38 & 99.21\textpm 0.39 & 98.66\textpm 0.38 \\ 
\hline
\multirow{3}{*}{Transformer} & Judg. & 96.86\textpm 0.17 & 97.80\textpm 0.16 & 95.94 0.25 & 96.92\textpm 0.36 & 97.86\textpm 0.19 & 96.01\textpm 0.62 \\
 & Laws & 89.48\textpm 0.57 & 91.63\textpm 0.75 & 87.43 0.65 & 97.15\textpm 3.73 & 97.55\textpm 3.78 & 96.74\textpm 3.68 \\
 & Laws + Judg. & 97.32\textpm 0.09 & 98.12\textpm 0.02 & 96.54 0.19 & 98.95\textpm 0.07 & 99.31\textpm 0.06 & 98.60\textpm 0.15 \\
\bottomrule
\end{tabular}
\end{table*}

\begin{table*}
\centering
\caption{Mean (\textpm std) performance of our models on the English dataset}
\label{tab:enTrained}
\begin{tabular}{c|c|c|c|c} 
\toprule
\multicolumn{1}{c}{} &  & \multicolumn{3}{c}{Judgements} \\
Model & Trained on & F1 & Precision & \multicolumn{1}{l}{Recall} \\ 
\midrule
CRF & Judg. & 98.76 & 98.84 & 98.69 \\
BiLSTM-CRF & Judg. & 97.34\textpm0.40 & 97.18\textpm0.56 & 97.51\textpm0.38 \\
Transformer & Judg. & 97.96\textpm0.08 & 97.84\textpm0.14 & 98.08\textpm0.13 \\
\bottomrule
\end{tabular}
\end{table*}

\begin{table*}
\centering
\caption{Mean (\textpm std) performance of our models on the German dataset}
\label{tab:deTrained}
\begin{tabular}{c|c|c|c|c|c|c|c} 
\toprule
\multicolumn{1}{c}{} &  & \multicolumn{3}{c|}{Judgements} & \multicolumn{3}{c}{Laws} \\
Model & Trained on & F1 & Precision & Recall & F1 & Precision & Recall \\ 
\midrule
\multirow{3}{*}{CRF} & Judg. & 97.77 & 98.12 & 97.43 & 76.51 & 96.50 & 63.38 \\
 & Laws & 75.82 & 78.68 & 73.16 & 97.67 & 97.88 & 97.47 \\
 & Laws + Judg. & 97.17 & 97.52 & 96.83 & 97.22 & 97.88 & 96.56 \\ 
\hline
\multirow{3}{*}{BiLSTM-CRF} & Judg. & 97.01\textpm 0.27 & 97.74\textpm 0.39 & 96.29\textpm 0.69 & 76.86\textpm 0.43 & 95.44\textpm 0.49 & 64.34\textpm 0.66 \\
 & Laws & 71.90\textpm 2.55 & 73.33\textpm 5.00 & 71.06\textpm 5.74 & 97.33\textpm 0.33 & 97.72\textpm 0.46 & 96.94\textpm 0.30 \\
 & Laws + Judg. & 97.16\textpm 0.20 & 97.36\textpm 0.44 & 96.97\textpm 0.57 & 97.56\textpm 0.16 & 98.34\textpm 0.16 & 96.78\textpm 0.23 \\ 
\hline
\multirow{3}{*}{Transformer} & Judg. & 97.96\textpm 0.23 & 98.08\textpm 0.13 & 97.84\textpm 0.35 & 87.18\textpm 0.43 & 96.05\textpm 0.33 & 79.82\textpm 0.56 \\
 & Laws & 89.40\textpm 0.51 & 93.04\textpm 0.98 & 86.04\textpm 1.05 & 97.44\textpm 0.05 & 97.37\textpm 0.12 & 97.51\textpm 0.12 \\
 & Laws + Judg. & 98.34\textpm 0.13 & 98.07\textpm 0.09 & 98.60\textpm 0.19 & 97.47\textpm 0.16 & 97.65\textpm 0.20 & 97.30\textpm 0.25 \\
\bottomrule
\end{tabular}
\end{table*}

\subsection{Performance of our multilingual models}
\label{ss:multilingualApp}

In Tables \ref{tab:multilingualBIG} and \ref{tab:zeroshot} we report the performance of our multilingual models on French, Spanish, Italian, English and German as well as their zero-shot performance on Portuguese.

\begin{table*}
\centering
\caption{Mean (\textpm std) performance of our multilingual models on French, Spanish, Italian, English and German}
\label{tab:multilingualBIG}
\resizebox{\textwidth}{!}{
\begin{tabular}{l|l|c|c|c|c|c|c|c|c|c} 
\toprule
\multicolumn{1}{l}{} & \multicolumn{1}{r|}{Language} & \multicolumn{2}{c|}{French} & \multicolumn{2}{c|}{Spanish} & \multicolumn{2}{c|}{Italian} & English & \multicolumn{2}{c}{German} \\
\hline
\multicolumn{1}{l}{} & \multicolumn{1}{r|}{Type} & Judg. & Laws & Judg. & Laws & Judg. & Laws & Judg. & Judg. & Laws \\
%\multicolumn{1}{l}{} &  & mean\textpm std & mean\textpm std & mean\textpm std & mean\textpm std & mean\textpm std & mean\textpm std & mean\textpm std & mean\textpm std & mean\textpm std \\
Model & Trained on &  &  &  &  &  &  &  &  &  \\ 
\midrule
\multirow{3}{*}{CRF} & Judg. & 97.4 & 93.3 & 95.7 & 96.5 & 97.9 & 77.3 & 95.7 & 95.0 & 72.1 \\
 & Laws & 89.8 & 98.3 & 63.6 & 98.4 & 84.1 & 98.3 & 69.2 & 75.2 & 94.0 \\
 & Laws + Jug & 97.8 & 98.1 & 94.8 & 98.9 & 97.3 & 97.7 & 95.1 & 95.2 & 91.6 \\ 
\hline
\multirow{3}{*}{BiLSTM-CRF} & Judg. & 97.9\textpm0.2 & 94.0\textpm0.8 & 97.0\textpm0.2 & 96.2\textpm0.7 & 97.7\textpm0.2 & 87.6\textpm0.8 & 95.6\textpm0.5 & 96.8\textpm0.2 & 76.5\textpm1.0 \\
 & Laws & 77.8\textpm0.9 & 98.4\textpm0.2 & 52.5\textpm2.6 & 99.0\textpm0.2 & 82.4\textpm1.7 & 98.9\textpm0.2 & 56.4\textpm1.9 & 74.2\textpm2.3 & \textbf{97.7}\textpm0.3 \\
 & Laws + Jug & 97.6\textpm0.3 & \textbf{98.5}\textpm0.2 & 97.3\textpm0.1 & \textbf{99.3}\textpm0.2 & 97.8\textpm0.1 & \textbf{99.2}\textpm0.1 & 95.4\textpm0.3 & 97.2\textpm0.2 & 97.5\textpm0.5 \\ 
\hline
\multirow{3}{*}{Transformer} & Judg. & \textbf{98.3}\textpm0.0 & 93.5\textpm1.1 & \textbf{97.8}\textpm0.1 & 97.7\textpm0.2 & 98.3\textpm0.1 & 85.5\textpm0.6 & 97.0\textpm0.1 & \textbf{98.4}\textpm0.1 & 86.7\textpm0.3 \\
 & Laws & 94.9\textpm0.4 & 98.3\textpm0.2 & 90.3\textpm1.2 & 99.0\textpm0.1 & 92.6\textpm0.4 & 99.1\textpm0.0 & 88.9\textpm0.8 & 89.3\textpm0.9 & 97.3\textpm0.1 \\
 & Laws + Jug & 98.3\textpm0.1 & 98.1\textpm0.2 & 97.8\textpm0.1 & 99.0\textpm0.0 & \textbf{98.3}\textpm0.1 & 99.1\textpm0.1 & \textbf{97.0}\textpm0.1 & 92.9\textpm0.2 & 97.6\textpm0.1 \\
\bottomrule
\end{tabular}}
\end{table*}



\begin{table*}
\centering
\caption{Mean (\textpm std) performance of our multilingual models on the unseen Portuguese dataset}
\label{tab:zeroshot}
\begin{tabular}{l|l|c|c|c|c|c|c} 
\toprule
\multicolumn{1}{l}{} & \multicolumn{1}{r|}{Type} & \multicolumn{3}{c|}{Judgements} & \multicolumn{3}{c}{Laws} \\
\hline
\multicolumn{1}{l}{} &  & F1 & Precision & Recall & F1 & Precision & Recall \\
%\multicolumn{1}{l}{} &  & mean\textpm std & mean\textpm std & mean\textpm std & mean\textpm std & mean\textpm std & mean\textpm std \\
Model & Trained on &  &  &  &  &  &  \\ 
\midrule
\multirow{3}{*}{CRF} & Judg. & 92.2 & 94.4 & 90.2 & 76.5 & 84.4 & 71.1 \\
 & Laws & 56.3 & 59.3 & 55.5 & 69.7 & 72.2 & 70.2 \\
 & Laws + Judg. & 90.2 & 91.7 & 88.8 & 78.6 & 88.2 & 71.5 \\ 
\hline
\multirow{3}{*}{BiLSTM-CRF} & Judg. & 92.5\textpm 1.5 & 93.9\textpm 0.8 & 91.2\textpm 3.0 & 78.5\textpm 4.0 & 93.4\textpm 2.3 & 68.5\textpm 5.8 \\
 & Laws & 46.1\textpm 1.5 & 58.2\textpm 5.8 & 38.8\textpm 4.3 & 76.2\textpm 3.2 & 91.7\textpm 3.8 & 66.2\textpm 4.9 \\
 & Laws + Judg. & 93.0\textpm 0.6 & \textbf{96.0}\textpm 0.8 & 90.4\textpm 1.3 & 73.2\textpm 3.3 & \textbf{97.2}\textpm 0.7 & 61.2\textpm 4.1 \\ 
\hline
\multirow{3}{*}{Transformer} & Judg. & \textbf{93.7}\textpm 0.3 & 93.5\textpm 0.3 & \textbf{93.8}\textpm 0.4 & \textbf{92.8}\textpm 0.2 & 93.7\textpm 0.7 & \textbf{91.9}\textpm 0.6 \\
 & Laws & 84.5\textpm 0.9 & 91.1\textpm 0.3 & 78.8\textpm 1.8 & 91.7\textpm 0.4 & 93.5\textpm 0.5 & 90.2\textpm 0.9 \\
 & Laws + Judg. & 93.6\textpm 0.3 & 93.6\textpm 0.4 & 93.5\textpm 0.2 & 91.3\textpm 1.1 & 94.2\textpm 0.5 & 88.8\textpm 1.7 \\
\bottomrule
\end{tabular}
\end{table*}

\fi
